# Supplementary material for: On the Parameterized Complexity of Odd Coloring
Source: arXiv:2503.05312 source file (2025-03-07)
Supplement: Supplementary file 1 [file appendix-star.tex]

\section*{Appendix}

\section{Proof of Lemma \ref{lem:rrs}}\label{app:tc}

Suppose $(G, k,t)$ is a yes-instance of \scp{}. Then it is easy to see that $(G-V(K'), k, t)$ is a yes instance of \scp{}. 
For the reverse direction, let $g$ be a star coloring of $(G-V(K'), k, t)$. 
We show how to extend $g$ to the vertices of $K'$ maintaining the star coloring requirement. 
We use  the colors from $g(K)$ (assigned to the vertices of $K$) to color the vertices of the deleted clique $K'\in K_A$. 
Every vertex in $K'$ is assigned a distinct color from $g(K)$. 
%in this process. 
This is possible as $|K'|\leq |K|$. 

We now prove that there is no bi-colored $P_4$ in $G$. 
Suppose not. Let there exist a bi-colored $P_4$ in $G$ because of the coloring assigned to $K'$. Notice that this happens 
only when there exists two vertices in $T_A$ that are assigned the same color. 
%{\color{red}
In this case, we would have applied our Claim \ref{cla:claim1}, which is a contradiction to the fact that $K_A$ does not satisfy the assumptions of Claim \ref{cla:claim1}.

\section{Clique-width Result from Section \ref{sec:cw}}\label{app:cw}

In this section, we show that \scp{} is FPT when parameterized by combined parameter
clique-width and the number of colors. We first give the definition of clique-width. 

%\textcolor{red}{
%1. l368-369 + abstract: announced like that, the result is a direct consequence of the theorem of CMR.
%You want to advertize the (improved) running time. (Probably the CMR paper should also be cited.) \\
%2. Please comment on MSO1 expressibility for your cliquewidth+k parameterization. \\
%3. In the case of cw, why don't you simply use the
%metatheorem, since the problem can be described in MSO1?}

\begin{definition}[Clique-width \cite{courcellecw}]
	Let $w \in \mathbb{N}$.
	A $w$-expression $\Phi$ defines a graph $G_\Phi$ where each vertex of $G$ receives a label from the set $[w]$,
	using the following four recursive operations with indices $i,j \in [w]$, $i\neq j$:

	\begin{enumerate}
	\item  Introduce, $\Phi=v(i)$: 
    $G_{\Phi}$ is a graph consisting a single vertex $v$ with label $i$. 
	\item Disjoint union,  $\Phi=\Phi' \oplus \Phi''$:   $G_{\Phi}$ is a disjoint union of the graphs $G_{\Phi'}$ and $G_{\Phi''}$. 
		
	\item  Relabel, {\bf $\Phi= \rho_{i\rightarrow j}(\Phi')$}:
	$G_\Phi$ is the graph $G_{\Phi'}$ where each vertex labeled $i$ in $G_{\Phi'}$ now has label $j$.
	\item Join, $\Phi=\eta_{i,j}(\Phi')$:
	$G_\Phi$ is the graph $G_{\Phi'}$ with additional edges between each pair of vertices $u$
	    of label $i$ and $v$ of label $j$.
	\end{enumerate}
The \emph{clique-width} of a graph $G$ denoted by \emph{cw(G)} is the minimum integer $w$
    such that there is a $w$-expression $\Phi$ that defines $G$. 
\end{definition}

Given a graph $G=(V,E)$ and an integer $k$, there is an FPT-algorithm that either reports $\operatorname{cw}(G) > w$ or outputs a $(2^{3w+2}-1)$-expression of $G$ \cite{DBLP:journals/jct/OumS06}. 
Hence, we assume that a $w$-expression $\Psi$ of $G$ is given. A $w$-expression $\Psi$ is a \emph{nice} $w$-expression of $G$, 
if no edge is introduced twice in $\Psi$. 
Given a $w$-expression of $G$, it is possible to get a nice $w$-expression of $G$ in polynomial time~\cite{courcellecw}.
For more details on clique-width we refer the reader to~\cite{hlinveny2008width}.

\medskip
\noindent
\textbf{Theorem \ref{thm:cw} (restated). }
Given a graph $G$, its nice $w$-expression and an integer $k$, we can decide if there exists a star coloring of $G$ using $k$ colors in $O((3^{w^3k^2+w^2k^2})^2 n^{O(1)})$ time.

%\textbf{Overview of the Algorithm:} 
\begin{proof}
Let $\Psi$ be a nice $w$-expression of the graph $G$. 
We give a dynamic programming algorithm over $\Psi$. 
 For each subexpression $\Phi$ of $\Psi$ and a coloring  $C:V(G_{\Phi}) \rightarrow [k]$ of $G_{\Phi}$,  we have a boolean table entry $d[\Phi;N;A;B]$ where 
$$N=n_{1,1},\dots n_{1,k},\dots, n_{w,1}, \dots n_{w,k}\mbox{, } $$
$$A=A_1, A_2, \dots, A_w,  \mbox{ where for each } i\in [w]  \mbox{ and } q,q'\in [k],$$
$$  A_i=\{A_{i,\{j,\ell\}}^{q,q'} \mid j,\ell\in [w]\mbox{ and }  j\neq \ell \}\cup \{A_{i, \{j,j\}}^{q, q'}
\mid j\in [w]\} \mbox{, and }$$
$$\mbox{for each } q,q'\in [k], B=\{B_{j, \ell}^{q,q'}\mid 
j, \ell\in [w] \}
$$

Given some vertex coloring of $G_\Phi$, we explain the meaning of each of the variables below. 

\noindent{}\textbf{N:} For each label $i\in [w]$ and color $q\in [k]$, the variable $n_{i,q}\in \{0,1,2\}$. Let $n_{i,q}^*$ denote the number of number of vertices with label $i$ and color $q$. Then $n_{i,q}=\max\{2, n_{i,q}^*\}$. The number of variables in $N$ is $wk$. 

\noindent{}\textbf{A:} Let $L=\{Y\subseteq [w] : |Y|=2\}$. 
%be the set of labels sets of size 2. That is $L={Y\subseteq [w]}\mid |Y|=2$. 
%The number of sets of labels from $[w]$ of size 2 is $\binom{w}{2}$. Let $L$ be the set of labels sets of size 2. 
That is $|L|=\binom{w}{2}$. 
For each label $i$ and set $\{j,\ell\}\in L$  or set $\{j, j\}\in L$ where $j, \ell\in [w]$,   the variable $A_{i,\{j,\ell\}}^{q,q'}\in \{0, 1, 2\}$. 
 Let $\widehat{A}_{i,\{j,\ell\}}^{q,q'}$ denote the number of vertices with label $i$ and color $q$ such that 
there exists two neighbors assigned the color $q'$, one with label $j$ and the other with label $\ell$. Then 
$A_{i,\{j,\ell\}}^{q,q'}= \max\{2, \widehat{A}_{i,\{j,\ell\}}^{q,q'}\}$. %From now on, we 
 Notice that the number of variables in $A$ is $k^2w(\binom{w}{2}+w)$.

\noindent{}\textbf{B:} 
%We use $L$, the set of label sets of size 2 in creating variables of $B$. 
%For each label set  $\{i,j\}\in L$ and pair of colors $q, q'\in [k]$, the variable $B_{\{i,j\}}^{q,q'}\in \{0, 1, 2\}$. 
For each pair of labels $i,j\in [w]$ and pair of colors $q, q'\in [k]$, the variable $B_{i,j}^{q,q'}\in \{0, 1, 2\}$. 
 Let $\widehat{B}_{i,j}^{q,q'}$ denote the number of vertices with label $i$ assigned the color $q$ such that 
there exists a neighbor  with label $j$ assigned the color $q'$. 
Then $B_{i,j}^{q,q'}= \max\{2, \widehat{B}_{i,j}^{q,q'}\}$. The number of variables in $B$ is $(wk)^2$. 

Note that for each $i, j, \ell\in [w]$ and colors $q, q'\in [k]$, 
the variable $A_{i,\{j,\ell\}}^{q,q'}$ (resp. $B_{i, j}^{q,q'}$) corresponds to the number of vertices, limited to a maximum of 2,  with label $i$ (resp. label $i$) adjacent to vertices with labels $j$ and $\ell$ (resp. label $j$) that are assigned the color $q'$. The primary difference between the variables is that the variables in $B$ are defined for each pair of labels $i,j\in [w]$ while the variables in $A$ are defined for each combination of $i$ and label set $\{j,\ell\}\in L$. 

 %u\in N(q')\in C(u) \mbox{ where }\}$
 
 For each subexpression $\Phi$ of $\Psi$, a boolean entry $d[\Phi;N;A;B]$ is set to TRUE if and only if 
 there is a vertex coloring $C:V(G_\Phi)\rightarrow[k]$ that satisfies the variables 
 $n_{i,q}$, $A_{i,\{j,\ell\}}^{q,q'}$ and $B_{i,j}^{q,q'}$ for each $i, j, \ell\in [w]$ and colors $q, q'\in [k]$. 
 If there is no coloring satisfying the variables entries in   $d[\Phi;N;A;B]$, then we set then the entry to FALSE.
We say that $G$ has a star coloring using $k$ colors if and only if there exists an entry $d[\Psi;N;A;B]$ that is set to TRUE. 
%where 
%for some $k$-star coloring of $G_{\Psi}$. 

We now give the details on how to compute an entry $d[\Phi;N;A;B]$ at each operation. 
\begin{enumerate}
  \item $\Phi=v(i)$. 
  
  $G_{\Phi}$ is the graph with one vertex $v$ with label $i$. The vertex $v$ could take any of the colors from $[k]$, and hence we set $k$ entries to be TRUE, one for each color. 
  That is, the entry $d[\Phi; N;A;B]$ is set to  TRUE if and only if 
  $n_{i, q}=1$ for each color $q\in [k]$ and all other variables of $N$, $A$ and $B$ are 0.

   \item $\Phi= \Phi' \oplus \Phi''$
   
       $G_{\Phi}$ is a  disjoint union of the graphs $G_{\Phi'}$ and $G_{\Phi''}$. 
       We set the entry $d[\Phi;N;A;B]$ to TRUE 
    if and only if there exist entries $d[\Phi';N';A';B']$
    and $d[\Phi''; N'';A'';B'']$
    such that both the entries are TRUE 
    and the following conditions hold:  
    \begin{enumerate}[label=(\roman*)]
        \item For each $i\in [w]$ and $q\in [k]$, 
        $n_{i,q}=\min\{2, n'_{i,q}+n''_{i,q} \}$.

    \item For each $i\in [w]$, set $\{j,\ell\}\in L$  and $q, q'\in [k]$, 
    $A_{i,\{j,\ell\}}^{q,q'}=\min\{2, A_{i,\{j,\ell\}}^{'q,q'}+A_{i,\{j,\ell\}}^{''q,q'}\}$. 
    
       \item For each $i, j\in [w]$,  and $q, q'\in [k]$, 
    $A_{i,\{j,j\}}^{q,q'}=\min\{2, A_{i,\{j,j\}}^{'q,q'}+A_{i,\{j,j\}}^{''q,q'}\}$.

    \item For each $i, j\in [w]$ 
    and $q, q'\in [k]$, 
    $B_{i,j}^{q,q'}=\min\{2, B_{i,j}^{'q,q'}+B_{i,j}^{''q,q'}\}$.

    %\item For each label $i\in [w]$ and pair of colors $q, q'\in [k]$, 
    %$B_{\{i,i\}}^{q,q'}=\min\{2, B_{\{i,i\}}^{'q,q'}+B_{\{i,i\}}^{''q,q'}\}$. 

    \end{enumerate}

   We now explain how to set an entry $d[\Phi;N;A;B]$ to TRUE. 
   Initially, we set all the entries in $G_\Phi$ to FALSE. 
   We consider all possible combination of entries $d[\Phi';N';A';B']$ and $d[\Phi'';N'';A'';B'']$ that are TRUE. 
   That is, for each pair of entries $d[\Phi';N';A';B']=$TRUE and $d[\Phi'';N'';A'';B'']$=TRUE, we update the corresponding entry $d[\Phi;N;A;B]$ satisfying the above conditions. 
    The number of such combinations is  $O((3^{w^3k^2+w^2k^2})^2)$ and we can compute the values of $N,A$ and $B$ in $O(w^3k^2)$ time. 
   
  \item  $\Phi=\rho_{i \rightarrow j} (\Phi')$.
  
	$G_{\Phi}$ is obtained from the graph $G_{\Phi'}$ by relabelling the vertices of label $i$ in $G_{\Phi'}$ with label $j$ where $i,j\in [w]$. 
	%Hence, $n_{i,q}=0$  for each $q \in [k]$, $B_{i,a}^{q,q'}=0$ for each label $a\in [w]$ 
	%and  
	%$A_{i,a,b}^{q,q'}=0$ for every label pair $a, b\in [w]$ and colors $q, q'\in [k]$. Note that the colors of the vertices remain unchanged in this process. 
	We set an entry $d[\Phi;N;A;B]$ to TRUE  if and only if there exists an entry $d[\Phi';N';A';B']$ in $G_{\Phi'}$ such that 
	$d[\Phi';N';A';B']$ is TRUE and the following conditions hold: 
	\begin{enumerate}[label=(\roman*)]
	    \item For each color $q\in [k]$ and
	    label $\ell\in [w]\setminus \{i,j\}$, 
			$n_{\ell,q}= n'_{\ell,q}$. 
	\item 	For each color $q\in [k]$,  
			$n_{j,q}= \min\{2, n'_{j,q}+n'_{i,q}\}$ and $n_{i,q}=0$.

			\item For each pair of colors $q, q'\in [k]$, the variables in $B$ are calculated as follows. 
			
%	\mybox{Hai}

	\noindent\fbox{
		\begin{minipage}{0.8\textwidth}
			\begin{tabular*}{\textwidth}{@{\extracolsep{\fill}}lr} \textbf{Computation of variables in $B$}  \\ \end{tabular*}
			\begin{itemize}
        			
	    \item For each pair of labels $a, b\in [w]\setminus \{i,j\}$,  
			$B_{a,b}^{q, q'}= B_{a,b}^{'q,q'}$.

       % \item For each label $a\in [w]\setminus \{i,j\}$, 
		%	$B_{\{a,a\}}^{q, q'}= B_{\{a,a\}}^{'q,q'}$. 

	\item 	For 
	each label $a\in [w]\setminus \{i,j\}$,  
			$B_{a,j}^{q,q'}= \min\{2, B_{a,j}^{'q,q'}+B_{a,i}^{'q,q'}\}$ and 
			$B_{j,a}^{q,q'}= \min\{2, B_{j,a}^{'q,q'}+B_{i,a}^{'q,q'}\}$.

	\item $B_{j,j}^{q,q'}= \min\{2, B_{j,j}^{'q,q'}+B_{i,i}^{'q,q'}+B_{i,j}^{'q,q'}+B_{j,i}^{'q,q'}\}$. 
			
			\item 	For each label $a\in [w]$,  $B_{a, i}^{q,q'}= 0$ and $B_{i,a}^{q,q'}= 0$. 
    \end{itemize}
		\end{minipage}
	}

		\item For each pair of colors $q, q'\in [k]$, the variables in A are calculated as follows. 	
			
%	\framebox[1.1\width]{This fits inside the frame}		
			
%\fbox{Hai
%\begin{minipage}{15em}
%Hello
%\end{minipage}
%}			

	\noindent\fbox{
		\begin{minipage}{0.8\textwidth}
			\begin{tabular*}{\textwidth}{@{\extracolsep{\fill}}lr} \textbf{Computation of variables in $A$}  \\ \end{tabular*}
		 \begin{itemize}

		\item For each $\ell, a, b\in [w]\setminus \{i,j\}$ and the set $\{a,b\}\in L$, 	
	    $A_{\ell,\{a,b\}}^{q,q'}=A_{\ell,\{a,b\}}^{'q,q'}$. 
	
	\item For each $\ell, a\in [w]\setminus \{i,j\}$, 
	$A_{\ell,\{a,a\}}^{q,q'}=A_{\ell,\{a,a\}}^{'q,q'}$. 				
						
		\item 	For   
		each $\ell, a\in [w]\setminus \{i, j\}$, 
	$A_{\ell,\{j,a\}}^{q,q'}=\min\{2, A_{\ell,\{i,a\}}^{'q,q'}+A_{\ell,\{j,a\}}^{'q,q'}\}$.

	\item 	For each $\ell \in [w]\setminus \{i, j\}$, 
	$A_{\ell,\{j,j\}}^{q,q'}=\min\{2, A_{\ell,\{j,j\}}^{'q,q'}+A_{\ell,\{i,j\}}^{'q,q'}+A_{\ell,\{i,i\}}^{'q,q'}\}$.

		\item 	For each $a, b\in [w]\setminus \{i, j\}$  and $\{a, b\}\in L$,  
	$A_{j,\{a,b\}}^{q,q'}=\min\{2, A_{j,\{a,b\}}^{'q,q'}+A_{i,\{a,b\}}^{'q,q'}\}$.

		\item 	For each $a\in [w]\setminus \{i, j\}$,  
	$A_{j,\{a,a\}}^{q,q'}=\min\{2, A_{j,\{a,a\}}^{'q,q'}+A_{i,\{a,a\}}^{'q,q'}\}$.

		\item For each $a\in [w]\setminus \{i, j\}$, 
		$A_{j,\{a,j\}}^{q,q'}=\min\{2, A_{j,\{a,j\}}^{'q,q'}+A_{i,\{a,j\}}^{'q,q'}+A_{j,\{a,i\}}^{'q,q'}+A_{i,\{a,i\}}^{'q,q'}\}$.

		\item $A_{j,\{j,j\}}^{q,q'}=\min\{2, A_{j,\{j,j\}}^{'q,q'}+A_{i,\{j,j\}}^{'q,q'}+A_{j,\{i,i\}}^{'q,q'}+A_{i,\{i,i\}}^{'q,q'}+A_{j,\{j,i\}}^{'q,q'}+A_{i,\{j,i\}}^{'q,q'}\}$. 
				
		\item For each $a, b, \ell\in [w]$, 
		$A_{\ell, \{a,b\}}^{q,q'}=0$ if  $a=i$ or $b=i$ or $\ell=i$. 
		
		\end{itemize}
		\end{minipage}
	}

	\end{enumerate}

	 	 We initially set each entry $d[\Phi;N;A;B]$ to be FALSE for each combination of $N, A$ and $B$. We consider all possible entries $d[\Phi';N';A';B']$ such that $d[\Phi';N';A';B']$ is TRUE and set the corresponding entry $d[\Phi;N;A;B]$ to TRUE based on the values computed using the above rules.  The number of entries to check is $O(3^{w^3k^2+w^2k^2})$ and we can compute the values of $N,A$ and $B$ in $O(w^3k^2)$ time.

 \item $\Phi=\eta_{i,j} (\Phi')$
 
$G_\Phi$ is obtained by connecting each vertex of label $i$ with each vertex of label $j$ in $G_{\Phi'}$. 
To ensure a proper coloring, we consider the entries 
$d[\Phi';N';A';B']$ that are set to TRUE in $G_{\Phi'}$ and has the property that, for each $q\in [k]$, 
if $n'_{i,q}\geq 1$ then $n'_{j,q}=0$ and vice-versa. 
%either $n'_{i,q}\geq 1$ or $n'_{j,q}\geq 1$ but not both. 
This condition ensures that the coloring obtained after the $\eta_{i,j}(\Phi')$ operation is indeed a proper coloring. 
It may be the case that $n'_{i,q}=0$ and $n'_{j,q}=0$, which implies that there are no vertices with labels $i$ and $j$ with the same color $q$. 

Before we proceed to the conditions on how to set an entry $d[\Phi;N;A;B]$ to TRUE, we look at each entry $d[\Phi';N';A';B']$ in $G_{\Phi'}$ that is set to TRUE and check if any of
the following four cases are met. The four cases are illustrated in Figure \ref{figure:star}.

\begin{figure}
\vspace{-0.3cm}
\begin{center}
\begin{tikzpicture}
[scale=0.5,auto=left, node/.style={circle,fill=white, draw, scale=0.5}
	,max/.style={circle,fill=black, draw, scale=1}]

	\node[node] (a1) at (-1,1) {};
	\node[node] (a2) at (-1,-2) {};
	\node[node] (a3) at (-4,1) {};
	\node[node] (a4) at (-4, -2) {};

	\node [above] at (a1.north) {$q'$};
	\node [above] at (a2.north) {$q'$};
	\node [above] at (a3.north) {$q$};
	\node [above] at (a4.north) {$q$};	
	\node [below] at (a1.south) {$j$};
	\node [below] at (a2.south) {$j$};
	\node [below] at (a3.south) {$i$};
	\node [below] at (a4.south) {$i$};

	\node[node] (b1) at (4,1) {};
	\node[node] (b2) at (4,-2) {};
	\node[node] (b3) at (6,-0.5) {};
	\node[node] (b4) at (2, -2) {};

	\node [above] at (b1.north) {$q$};
	\node [above] at (b2.north) {$q$};
	\node [above] at (b3.north) {$q'$};
	\node [above] at (b4.north) {$q'$};	
	\node [below] at (b1.south) {$i$};
	\node [below] at (b2.south) {$i$};
	\node [below] at (b3.south) {$j$};
	\node [below] at (b4.south) {$a$};

		\node[node] (c1) at (11,1) {};
	\node[node] (c2) at (11,-2) {};
	\node[node] (c3) at (9,-0.5) {};
	\node[node] (c4) at (13, -2) {};

	\node [above] at (c1.north) {$q'$};
	\node [above] at (c2.north) {$q'$};
	\node [above] at (c3.north) {$q$};
	\node [above] at (c4.north) {$q$};	
	\node [below] at (c1.south) {$j$};
	\node [below] at (c2.south) {$j$};
	\node [below] at (c3.south) {$i$};
	\node [below] at (c4.south) {$a$};

	\node[node] (d1) at (-1,-6) {};
	\node[node] (d2) at (0,-7) {};
	\node[node] (d3) at (-4,-6) {};
	\node[node] (d4) at (-5, -7) {};

	\node [above] at (d1.north) {$q'$};
	\node [above] at (d2.north) {$q$};
	\node [above] at (d3.north) {$q$};
	\node [above] at (d4.north) {$q'$};	
	\node [below] at (d1.south) {$j$};
	\node [below] at (d2.south) {$b$};
	\node [below] at (d3.south) {$i$};
	\node [below] at (d4.south) {$a$};

		\node[node] (e1) at (5,-6) {};
	\node[node] (e2) at (7,-6) {};
	\node[node] (e3) at (3,-6) {};
	\node[node] (e4) at (2, -7) {};

	\node [above] at (e1.north) {$q$};
	\node [above] at (e2.north) {$q'$};
	\node [above] at (e3.north) {$q'$};
	\node [above] at (e4.north) {$q$};	
	\node [below] at (e1.south) {$i$};
	\node [below] at (e2.south) {$j$};
	\node [below] at (e3.south) {$a$};
	\node [below] at (e4.south) {$b$};

		\node[node] (f1) at (13,-6) {};
	\node[node] (f2) at (14,-7) {};
	\node[node] (f3) at (11,-6) {};
	\node[node] (f4) at (9, -6) {};

	\node [above] at (f1.north) {$q$};
	\node [above] at (f2.north) {$q'$};
	\node [above] at (f3.north) {$q'$};
	\node [above] at (f4.north) {$q$};	
	\node [below] at (f1.south) {$a$};
	\node [below] at (f2.south) {$b$};
	\node [below] at (f3.south) {$j$};
	\node [below] at (f4.south) {$i$};

	\node [above] at (-2.5,-4) {(a) Case 1};
	\node [above] at (4.5,-4) {(b) Case 2(i)};
	\node [above] at (10.5,-4) {(c) Case 2(ii)};
	\node [above] at (-2.5,-9) {(d) Case 3};
	\node [above] at (4.5,-9) {(e) Case 4(i)};
	\node [above] at (10.5,-9) {(f) Case 4(ii)};

	\draw (a1) -- (a3) -- (a2) -- (a4); 
	\draw (b1) -- (b3) -- (b2) -- (b4); 
	\draw (c1) -- (c3) -- (c2) -- (c4); 
	\draw (d2) -- (d1) -- (d3) -- (d4); 
	\draw (e2) -- (e1) -- (e3) -- (e4); 
    \draw (f2) -- (f1) -- (f3) -- (f4);

\end{tikzpicture}
\end{center}
\vspace{-0.3cm}
\caption{Various cases of bicolored $P_4$ that may arise out of the operation $\Phi=\eta_{i,j}(\Phi')$. Each vertex is represented by $\circ$, where its label and color are represented by the values below and above ``$\circ$'' respectively.  }
\label{figure:star}
\vspace{-0.5cm}
\end{figure}

 \begin{itemize}

     \item \textbf{Case 1:} There exists a pair of colors $q, q'\in [k]$ such that $n'_{i, q}=2$ and $n'_{j,q'}=2$.

     \item \textbf{Case 2:} There exists a pair of colors $q, q'\in [k]$ and label $a\in [w]\setminus \{i,j\}$ 
     such that either (i) 
     $n'_{i, q}= 2$,  $n'_{j,q'}= 1$ and $B_{i,a}^{'q,q'}\geq 1$,  
     or 
     (ii) $n'_{i, q}= 1$,  $n'_{j,q'}= 2$ and $B_{j,a}^{'q',q}\geq 1$.

    \item \textbf{Case 3:} There exists a pair of colors 
    $q, q'\in [k]$ and labels $a, b\in [w]\setminus \{i, j\}$ 
    such that $n_{i,q}=1$, $n_{j,q'}=1$, 
     $B_{i,a}^{'q, q'}\geq 1$ and $B_{j,b}^{'q',q}\geq 1$. 
    % Note that $a\neq b$ in this case. Else we do not have a proper coloring. 

     \item \textbf{Case 4:} There exists a pair of colors 
    $q, q'\in [k]$ and  labels $a, b\in [w]\setminus \{i,j\}$  
    such that $n_{i,q}=1$, $n_{j,q'}=1$, 
     and either $A_{a, \{i,b\}}^{'q', q}\geq 1$ 
     or 
     $A_{a, \{j,b\}}^{'q, q'}\geq 1$. 
     %Note that $a\neq b$ in this case, else there we do not have a proper coloring. 

\end{itemize}
 
We consider only those entries $d[\Phi';N';A';B']$ that are set to TRUE and do not satisfy any of the above four cases. 
If an entry satisfies any of the above four cases, then the $\eta_{i,j}(\Phi')$ results in a bi-colored $P_4$ 
and hence it is 
not considered for further processing. 
If none of the above cases are met, then we consider the entry $d[\Phi';N';A';B']$ that is set to TRUE  for further processing. %This is because the $\eta_{i,j}(\Phi')$ 
% operation on $d[\Phi';N';A';B']$ 
% will not create must not yield a bi-colored $P_4$. 

We set an entry $d[\Phi;N;A;B]$ to be TRUE  if and only if there exists an entry $d[\Phi';N';A';B']$ 
in $G_{\Phi'}$ such that 
	$d[\Phi';N';A';B']$ is set to TRUE, not satisfying any of the above four cases 
	and the following conditions are met: 

    \begin{enumerate}[label=(\roman*)]
        \item  For each $q\in [k]$ and
	  $a\in [w]$, 
			$n_{a,q}= n'_{a,q}$. 
			
	    \item  For each $q, q'\in [k]$ and 
	    $a \in [w]\setminus \{i,j\}$, $b\in [w]$, 
			$B_{a,b}^{q,q'}= B_{a, b}^{'q,q'}$.

			 \item  For each $q, q'\in [k]$ and
	    $a \in [w]\setminus \{j\}$, $b\in [w]\setminus \{i\}$, 
	    $B_{i, a}^{q,q'}= B_{i, a}^{'q,q'}$ and $B_{j, b}^{q,q'}= B_{j, b}^{'q,q'}$.  
	    
	    \item For  each $q, q'\in [k]$, we have  $B_{i,j}^{q,q'}=\min\{2,n'_{i,q}\}$ if $n'_{j,q'}\geq 1$ 
	    and $B_{i,j}^{q,q'}=0$ otherwise. 
	    Similarly, we have 
	    $B_{j,i}^{q,q'}=\min\{2, n'_{j,q}\}$ if $n'_{i,q'}\geq 1$ and 
	    $B_{j,i}^{q,q'}=0$ otherwise. Note that $B_{i,j}^{'q,q'}=0$ and $B_{j,i}^{'q,q'}=0$ in $G_{\Phi'}$ because $\Phi'$ is a nice $w$-expression of $G_{\Phi'}$. 
	    
	   		\item For each pair of colors $q, q'\in [k]$, we compute the variables in $A$ as follows:

	\noindent\fbox{
		\begin{minipage}{0.8\textwidth}
			\begin{tabular*}{\textwidth}{@{\extracolsep{\fill}}lr} \textbf{Computation of variables in $B$}  \\ \end{tabular*}
		 \begin{itemize}
        \item For each label set  $\{a, b\}\in L$ and $\ell\in [w]\setminus \{i,j\}$, we have 
	    $A_{\ell, \{a, b\}}^{q,q'}=A_{\ell, \{a, b\}}^{'q, q'}$.
	    	    
	  \item For each $a\in [w]$ and $\ell\in [w]\setminus \{i,j\}$, 
	   $A_{\ell, \{a, a\}}^{q,q'}=A_{\ell, \{a, a\}}^{'q, q'}$.

	  \item For each label set $\{a, b\}\in L$ and $a, b\in [w]\setminus \{j\}$, 
	   $A_{i,\{a,b\}}^{q,q'}=A_{i,\{a,b\}}^{'q,q,'}$. Also for each $a\in [w]\setminus \{j\}$, $A_{i,\{a,a\}}^{q,q'}=A_{i,\{a,a\}}^{'q,q,'}$.

	 \item For each label set $\{a, b\}\in L$ and $a, b\in [w]\setminus \{i\}$, 
	   $A_{j,\{a,b\}}^{q,q'}=A_{j,\{a,b\}}^{'q,q,'}$.   
	   Also for each $a\in [w]\setminus \{i\}$, $A_{j,\{a,a\}}^{q,q'}=A_{j,\{a,a\}}^{'q,q,'}$.
	   
	 \item For each label $a \in [w]\setminus \{j\}$, we have $A_{i,\{j,a\}}^{q,q'}=0$ if $n'_{j,q'}=0$. 
	 Else we have 
	    $A_{i,\{j,a\}}^{q,q'}=B_{i,a}^{'q,q'}$. 
	    %Note that $B_{i,a}^{q,q'}=B_{i,a}^{'q,q'}$. 
	    
	    \item For each label $a \in [w]\setminus \{i\}$, we have $A_{j,\{i,a\}}^{q,q'}=0$ if $n'_{i,q'}=0$. 
	 Else we have 
	    $A_{j,\{i,a\}}^{q,q'}=B_{j,a}^{'q,q'}$. 
	    %Note that $B_{j,a}^{q,q'}=B_{j,a}^{'q,q'}$. 

%	    \item For each color pair $q,q'\in [k]$, 
%	    label $a \in [w]\setminus \{i\}$ and 
%	    if $n_{i,q'}=0$ we have $A_{j, i, a}^{q,q'}=0$ and $A_{j, i, a}^{q,q'}=0$, else we have 
%	    $A_{j,i,a}^{q,q'}=B_{j,a}^{q,q'}$ and $A_{j,a,i}^{q,q'}=B_{j,a}^{q,q'}$. 

	    \item $A_{i,\{j,j\}}^{q,q'}=n'_{i,q}$ if $n'_{j,q'}=2$ and $A_{i,\{j,j\}}^{q,q'}=0$ otherwise. 
	    \item 
	    $A_{j,\{i,i\}}^{q,q'}=n'_{j,q}$ if $n'_{i,q'}=2$ and $A_{j,\{i,i\}}^{q,q'}=0$ otherwise. 
			
   \end{itemize}
		\end{minipage}
	}

    \end{enumerate}
    			
		We initially set all the entries in $G_\Phi$ to be FALSE. For each TRUE entry $d[\Phi';N';A';B']$, we check if all the above conditions are met (besides not falling into any of the four cases) and then assign the respective entry $d[\Phi;N;A;B]$ to be TRUE. 
	    The number of entries to check is $O(3^{w^3k^2+w^2k^2})$ and we can compute the values of $N,A$ and $B$ in $O(w^3k^2)$ time.

\end{enumerate}	   
    The correctness of the algorithm follows from the description of the algorithm. The time taken by the algorithm is $O((3^{w^3k^2+w^2k^2})^2n^{O(1)})$. 
%\qed
%\end{proof}

\qed
\end{proof}

\section{Co-cluster}

% \subsection{Old}
\begin{proof}
 Let $X \subseteq V(G)$ of size $t$ be  such that $G -X$ is a complement of cluster. That is, 
 $G-X$ is partitioned into independent sets $I_1, I_2, \dots, I_p$ such that 
 each vertex in $I_i$ is adjacent to every vertex in $I_j$, for all $i\neq j$.

 The algorithm is similar in flavor to the one in Theorem \ref{thm:cvd}. 
 We highlight the key steps below. 
 \begin{itemize}
     \item After we guess the functions $f$ and  $g$ for the set $X$, we 
     guess the set of colors from $[t']$ that are assigned to the vertices in the independent sets of $G-X$. Since it  is a proper coloring, each color from $[t']$ is assigned to vertices of at most one independent set. 
     \item However a color from $[t']$ can be assigned to multiple vertices in the independent type. We partition the vertices of each independent types based on its neighbors in $X$. 
     We guess the set of types that the vertices in the independent type are assigned a color $c\in [t']$. In addition, we guess the parity of the color in each independent type.

         For a subset $Y \subseteq X$, we define  $T^Y_I$ to be the set of vertices of an independent type $I$ such that each vertex for $v\in T^Y_I$, we have $N(v)\cap X=Y$. 
     %$=\bigcup\limits_{I}T^Y_I$. 
   
   For each $Y \subseteq X$, let $h^Y: [t'] \rightarrow \{e,o,0\}$, where $h^Y(i)$ denotes the 
 parity of color $i$ in $T^Y_I$, for some $I$. 
 Let $h=\{h^Y~|~Y \subseteq X\}$.

     \item Each color from $[t']$ can be assigned to at most one independent type. We guess the set of colors from $[t']$ that are assigned to vertices in an independent type. Notice that there are at most $t'$ many independent sets where vertices are assigned colors from $[t']$. Let $z:[t']\rightarrow [t^*]$ be the function that assigns the colors from $[t']$ to $t^*$ independent types. Let $\mathcal{Z}=\{Z_1, Z_2, \dots, Z_{t^*}\}$ be hypothetical independent sets such that the colors that are assigned to $Z_i$ is the set $z^{-1}(i)$. 
     %be the set if colors that are assigned to an independent type. That is $z_i$

        \item 
     As a result of this, all vertices in $X$ have an odd color. Some vertices of $G-X$ may not have an odd color. 
     Let $\ell$ be the number of independent types that contains an vertex that is not yet assigned a color. 
     From Lemma \ref{lem:q+2-dcoc}, 
     we get that at most $\ell+2$ colors are sufficient to color the $\ell$ independent sets and ensure that every vertex in $G-X$ also has an odd color.

    \item Notice that $\ell$ colors are required for a proper coloring of these independent types respecting $(c, q, \mathcal{Z})$. We guess whether one or two extra colors are needed. If two extra colors are 
     needed, 
     say $\widehat{c}$ and $c^*$, 
     then we guess the  independent types $\widehat{I}$ and $I^*$ 
     that contains a vertices of the colors $\widehat{c}$ and $c^*$. 
     In addition we also guess the parity of $\widehat{c}$ in each of the types of $\widehat{I}$. We preform the same for $I^*$. Now every vertex in $G$ has an odd color. We now use the extension of the coloring using Lemma \ref{lem:colo-ex-coc}. 
     \item The last step is to identify the independent sets in $\mathcal{Z}$ from $I_1, I_2, \dots, I_p$ using a dynamic programming routine using the above guess. 
     
     %Each uncolored vertex in an independent set can be assigned a new color. 

   %   To tackle these vertices at most two vertices 
     %receives a color  
 \end{itemize}

\begin{proof}[Proof of Lemma \ref{lem:colo-ex-coc}]
We first try to extend the coloring using the colors that are used in the precoloring. Without  loss of generality, let the colors used be 
$[t']\cup \{\widehat{c}, c^*\}$.

For an independent type $I_q \in G-X$, let 
   \begin{itemize}
       \item $I_q$ be the independent type $Z_i$, for some $i$, and  
       \item the set of hypothetical types among the independent types $I_1\cup \dots \cup I_q$ is $\widehat{Z}_i$ and  $Z_i\in \widehat{Z}_i$. 
       
%       $h^{Y}_q: [t'] \rightarrow \{e,o,0\}$, where 
%   $h^{Y}_q(i)$ 
%   denotes the  parity of a color $i\in [t']$ in $T^Y_{C_q}$. 
%   \item   $\widehat{h}^Y_q:[t'] \rightarrow \{e,o,0\}$, where $\widehat{h}^Y_q(i)$ denotes the parity of color $i$ in $\bigcup \limits _{j \in [q]} T^Y_{C_j}$. 
%   \item  
   %For $q \in [p]$ and a clique $C$, 
   %let 
%   $h_q=\{h^{Y,C}_q~|~Y \subseteq X\}$ and $\widehat{h}_q=\{\widehat{h}^Y_q~|~Y \subseteq X\}$.

   \end{itemize}
   \medskip 
\noindent
\emph{Definition of the table entry.} For a tuple $(k,Z_i,\widehat{Z}_i)$, 
let $M[k, Z_i, \widehat{Z}_i]$ 
denote the minimum number of new colors (outside $[t']\cup \{\widehat{c}, c^*\}$) 
 needed to color the graph $G[I_1, \dots, I_k]$ such that 
 %for a subset $Y \subseteq X$, 
 \begin{itemize}
  \item $I_k$ is the set $Z_i$, 
and the set of colors used in $I_k$ is $z^{-1}(i)$ and the parity of each color $s\in z^{-1}(i)$ is $h^Y(s)$, for each $Y\subseteq X$, 
\todo[]{Check for the colors $\widehat{c}, c^*$}

  \item the hypothetical sets $\widehat{Z}_i\subseteq \{I_1,  \dots , I_{k}\}$.  
%  \item the parity of a color $i$, in $T^Y_{C_k}$ is $h^{Y}_k(i)$, 
%  \item for a subset $Y \subseteq X$, the parity of a color $i$, in $\bigcup \limits _{j \in [k]} T^Y_{C_j}$  is $\widehat{h}^Y_k(i)$, and 
%  \item each of the vertices in the cliques $C_1, \dots, C_k$ has an odd color. 
 \end{itemize}

Consider $T^Y_{I_k}$, where $Y\subseteq X$. We have the following cases. Let $t^Y_{I_k}$ denote the number of vertices from $T^Y_{I_k}$ that are not assigned a color. 

\begin{itemize}
\item \textbf{$|T^Y_{I_k}|-t^Y_{I_k}$ is even. }

    \begin{itemize}
       \item \textbf{There exists a vertex in $T^Y_{I_k}$ that is assigned a color $d$. }

       Assign $d$ to the remaining unassigned vertices of $T^Y_{I_k}$. The parity of $d$ does not change because of the case assumptions. 

       \item \textbf{There exists a vertex in $T^Y_{I_k}$ that is assigned a color $d$. }

       We cannot use the existing color and we need a new color. 
       
    \end{itemize}
    \item \textbf{$|T^Y_{I_k}|-t^Y_{I_k}$ is odd. }
    \begin{itemize}
        \item \textbf{There exists a vertex in $T^Y_{I_k}$ that is assigned a color $d$. }

        Assign all but one unassigned vertex of $T^Y_{I_k}$ the color $d$. The parity of $d$ does not change because of the case assumptions. 

        \item \textbf{There exists a vertex in $T^Y_{I_k}$ that is assigned a color $d$. }

       We cannot use the existing color and we need a new color. 
           \end{itemize}
\end{itemize}
We repeat this process for each $Y\subseteq X$ in the independent set $I_k$. After processing all the independent types in the above fashion, we ensured that all the uncolored vertices should receive a new color (other than $[t']\cup \{\widehat{c}, c^*\}$). Notice that all these vertices can be assigned the same color. 

We now show how to compute the entry $M[k, Z_i, \widehat{Z}_i]$. 
We set $M[k,  Z_i, \widehat{Z}_i]=\infty$
if any of the above conditions does not hold. Else, 
$$M[k, Z_i, \widehat{Z}_i]=a_k+T[k-1,*, \widehat{Z}_i\setminus Z_i\}$$ 
where $a_k\in \{0,1\}$. We assign  
$a_k=1$ if there exists an unassigned vertex in $I_k$ after the extension, and $a_k=0$ otherwise. 
    \qed
\end{proof}
This completes the proof. 
\qed
\end{proof}
% \subsection{Old}
% \begin{itemize}
%     \item Guess a coloring $f:S\rightarrow [\ell]$ of $S$ that appears in an odd coloring of $G$, where $\ell<t$. 
%     We first extend the coloring $f$ to a partial coloring of $V(G)$ using the color from $\{1, 2, \dots, \ell\}$. 

%     \item Any color $c$ that is used outside $S$, can be used in at most one independent set. 

%         \item We guess the partitions of vertices of  $S$ that have the same odd color. 
%     Since we may need a new odd color for each vertex in $S$, combined with the colors used for $S$, 
%     there are at most $2t$ many partitions. 
%     For each of the partitions that do not correspond to the colors $\{1, 2, \dots, \ell\}$, we introduce a new color. Let the colors be $\{1, 2, \dots, \ell, \dots, t'\}$.  
%     \item For each type $A\subseteq S$, we guess whether a color from $[t']$ appears odd or even number times across all the cliques of they type. 
% \item In addition to this, we know that at most two colors (one in each independent set) are sufficient to ensure an odd color for each vertex in $G-S$. We guess the independent sets that contain these two colors and also the type and appearance of even or odd number of times in that type. 

% \item The next step is a dynamic programming based algorithm on the independent sets (similar to the distance to cluster dp) that finds the number of new colors required for a
    
% \end{itemize}
